# Supplementary material for: SkyStore: Cost-Optimized Object Storage Across Regions and Clouds
Source: arXiv:2502.20818 source file (2025-02-28)
Supplement: Supplementary file 1 [file Appendix.tex]

\newpage
\newpage
\begin{figure*}[tbp]
    \centering
    \includegraphics[width=\textwidth]{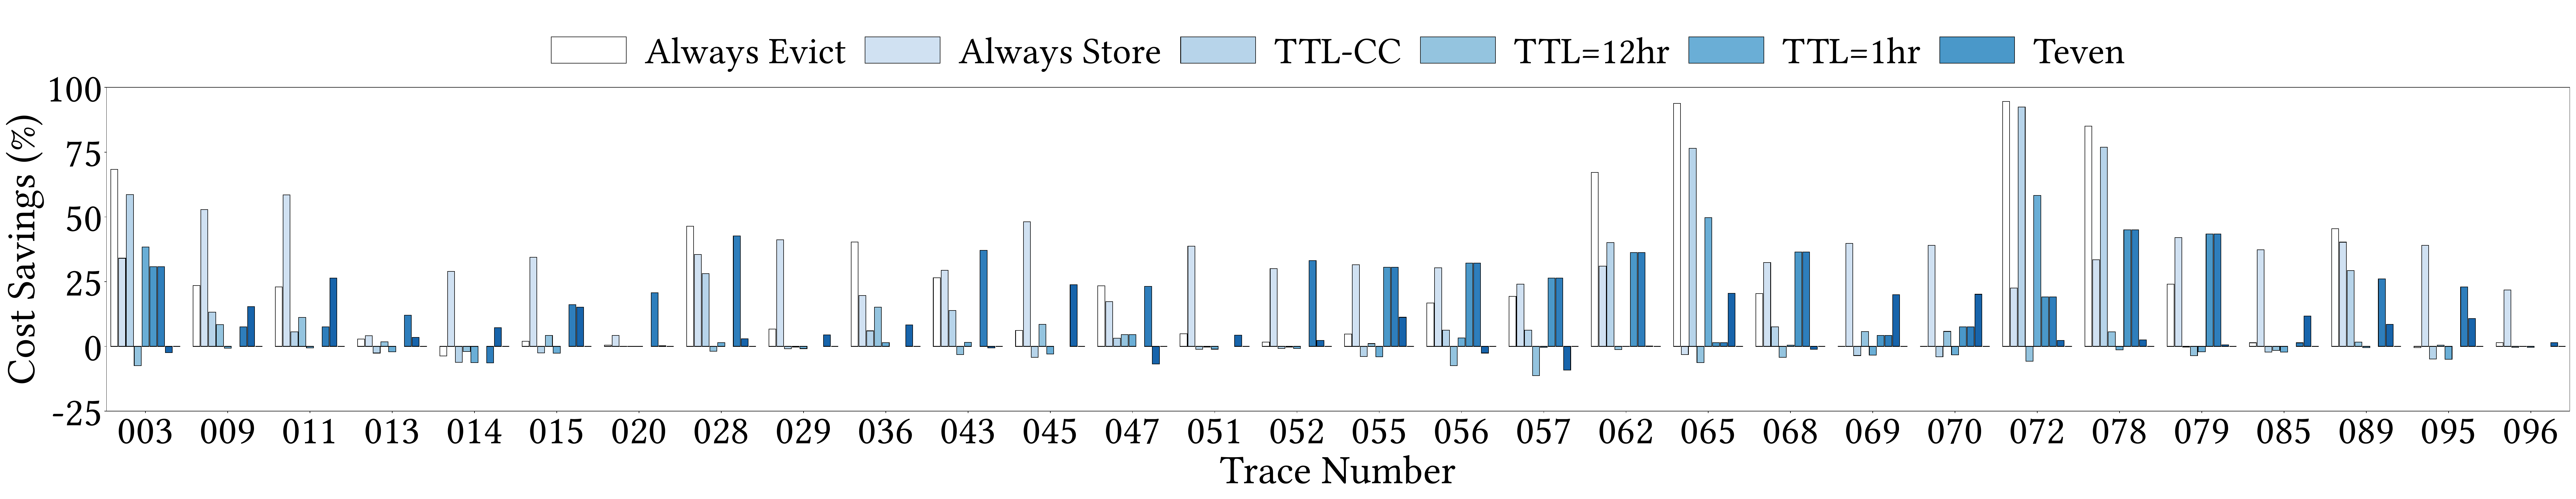}
    % \vspace{-2em}
    \caption{\textbf{\sys Cost Savings (\%) on 7-Region, Free Placement (FP)}: \sys achieves on average 1\%-61\% cost savings over over 30 traces and 6 other baselines.}
    \label{fig:7-region-fp}
\end{figure*}

\begin{figure*}[tbp]
    \centering
    \includegraphics[width=\textwidth]{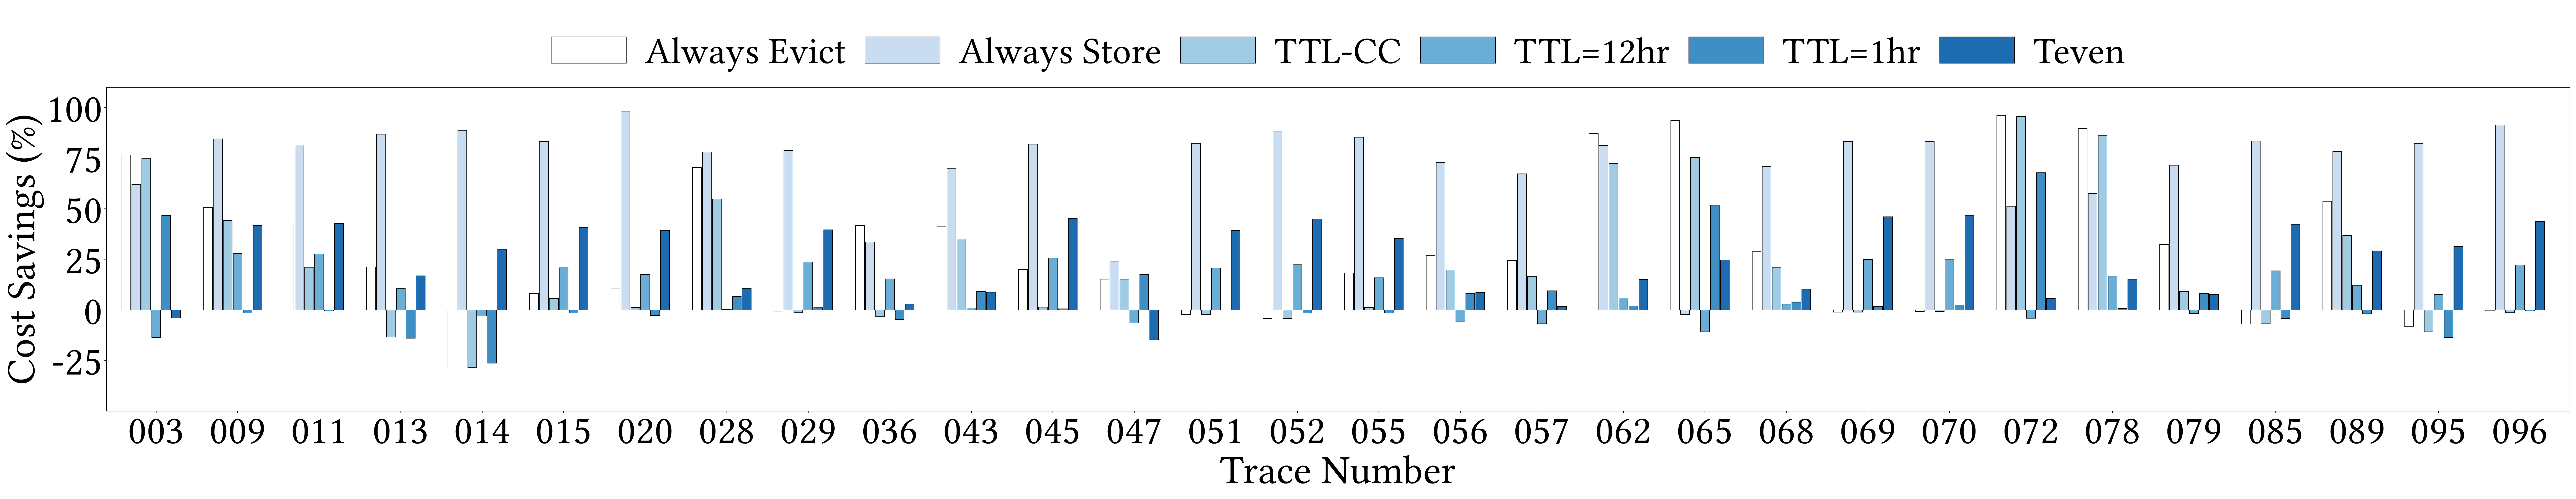}
    % \vspace{-2em}
    \caption{\textbf{\sys Cost Savings (\%) on 9-Region, Fixed Base (FB)}: \sys achieves on average 12.1\%-69.3\% cost savings over over 30 traces and 6 other baselines.}
    \label{fig:9-region-fb}
\end{figure*}

\section{Optimal vs.\ Break-Even Policies }\label{s:appendix}
This appendix refers to a two-site caching problem in which one site is the base and the second is the cache site. 
Costs account for storage at the cache site (not the base site), and all network costs from the base to the cache. 

We measure ourselves against a {\em Clairvoyant} policy that is given access to an {\em oracle} that knows exactly when an object will be read in the future (if at all). This is the equivalent of Belady's algorithm but adapted to the different settings of our caching problem. Every time an object is read, the optimal policy compares the time for next access $T_{\text{next}}$ with the break-even time $T_{\text{even}}$. If $T_{\text{next}} > T_{\text{even}}$, it immediately evicts the object, as it is more costly to keep the object around as opposed to reading it again from a distant location. Otherwise, the optimal strategy keeps it in the cache.  This strategy is proved to be optimal in \cite{TTLbasedCC2019} for a two-site base and cache setting. Recall that $\teven$ is chosen to be the time for which $\teven \cdot S = N$.
Consider the $\teven$-policy that sets $\tev = \teven$. We show that when compared to the optimal clairvoyant strategy, the cost of the  $\teven$-policy is no more than double.  

The cost per byte for a single object in the {\bf optimal policy} is:
$$ \sum_{i| \tnext(i) \leq \teven} \tnext(i) \cdot S + \sum_{i| \tnext(i) > \teven} N  + N $$
The last $N$ is the cost of the initial GET, whereas there is no cost after the last get as the object is evicted. 

%The {\bf $\tev$ policy} evicts items after $\tev$ time has passed since their last access. The cost of this policy is (per byte per single object):
%$$ \sum_{i| \tnext(i) \leq \tev} \tnext(i) \cdot S + \sum_{i| \tnext(i) > \tev} (N+\tev\cdot S) + (N+\tev\cdot S)$$
%The last $(N+\tev\cdot S)$ includes the cost of the initial GET as well as the cost of keeping the object around after the last GET. 

 The cost of the $\teven$-policy policy is:
$$ \sum_{i| \tnext(i) \leq \teven} \tnext(i) \cdot S + \sum_{i| \tnext(i) > \teven} 2N + 2N$$
The last $2N$ includes the cost of the initial GET and the cost of keeping the object around after the last GET.

The first part is identical, whereas the second part is exactly double that of the optimal cost. 
Namely, the cost of the $\teven$ policy is bounded by $2 X$ that of the optimal algorithm.

On the other hand we claim that for every eviction strategy there exists an (adversarially chosen) workload for which the cost amount to more than twice that of the optimal strategy. 
This can be shown for each object separately. It starts by reading the object once (therefore putting it in the cache). If the eviction policy P decides to evict the object after more than $\teven$ time, then the workload never asks for this object again. 
In such a case, the optimal strategy cost would be $N$ (just for the first GET), whereas the cost for policy $P$ would be greater than $N + \teven \cdot S = 2N$.

 If, on the other hand, P decides to evict the object earlier, at time $t < \teven$, then the workload submits a GET after $t + \varepsilon$ time, subject to $t + \varepsilon<\teven$. 
 The $\co$ in this case is $N+(t+\varepsilon)\cdot S$ whereas for $\cp$ is $2N+t\cdot S$.
 Since the object is in the cache again, we recursively continue.
 After $k$ iterations we have $\co = N+(\sum (t_i+\varepsilon))S$ whereas $\cp = (k+1)N + (\sum t)S$.
 
 The difference between them is  $\cp - \co = kN + k\varepsilon$ since $\co <(k+1)N$ then choose $k$ to be large enough so that $k \varepsilon> N$ which will cause $\cp-\co > \co$ and give us a ratio $\geq 2$.

\section{Adding Latency Considerations - Pricing Hits}\label{app:hits}
An alternative approach to putting a price tag on cache misses is pricing hits. Namely to ask how much a customer is willing to pay for cache hits. If all things are equal, how much additional cost the user would be willing to pay for getting local latency and bandwidth? Call this value a {\em user performance value}, denoted by $\uval$, and it is a cost per byte.
We add this to the basic methodology of choosing a $\ttl$ as follows: After finding the value of $\ttl$ that achieves the lowest expected cost, check whether there is a higher $\ttl$ value for which the average cost per additional hit is bounded by the $\uval$. 

More formally, let $\ttl'$ stand for the eviction time, achieving the best expected cost. We choose the highest value $\ttl$ such that 
$$ \frac{ExpectedCost(\ttl) - ExpectedCost(\tev')}{\text{object byte count between $\tev$ and $\tev'$}} \leq \uval$$ 

For each cached object, the user pays the storage for this cache until the time $T$ of the next read or eviction. This amounts to $T \times \text{Size}(o) \times S$.

%%%%%%%%%%%%%%%%%%%%%%%%%%%%%%%%%%%%%%%%%%%%%%%%%%%%%%%%%%%%
% Danny - all of the below is text that was removed from various versions of the eviction policy
%
\remove{
\subsubsection{Pull-based policy with eviction}
\textbf{Decision} Whether to evict or keep object $o$ in region $r$ \newline \newline
\textbf{Input}
\begin{enumerate}
    \item Past history of access to this object $o$ in region $r$
    \item Storage cost per region: $\$$/GB per time
    \item Egress cost between regions: $\$$/GB
    \item $\text{Replica(}o\text{)}$: set of regions storing the replicas, including $r$
    \item $\text{Size(}o\text{)}$ = size of object in GB 
\end{enumerate}
\subsubsection{Expected time for next access}\danny{Need to decide if this is relevant or do we remove the attempt to predict $\tnext$.}
\begin{equation}
T_{\text{next}}(o,r) = \alpha \times T_{\text{current}}(o,r) + (1-\alpha) \times T_{\text{previous}}(o,r)
\end{equation}

% max of accesses to these objects not very large, relatively short time 
% read only once, read once a day 
% identify that 95% that is read once, won't cache any thing (5%) - type A, B
Where:

\begin{itemize}
\item \( T_{\text{next}}(o,r) \) is the expected time of the next access of object \( o \) in region \( r \).
\item The calculation uses the Exponentially Weighted Moving Average (EWMA) method.
\item \( \alpha = 0.5 \)
\item \( T_{\text{current}}(o,r) \) denotes the time since the last access for object \( o \) in region \( r \).
\item \( T_{\text{previous}}(o,r) \) denotes the previously computed expected value.
\item Initialization can be done using the average of the initial intervals. For instance, if access times are at 1, 4, and 6, the time intervals are 3 and 2. The average is \( \frac{5}{2} = 2.5 \).
\end{itemize}

% \danny{The initialization part is tricky. Consider a new object that is read for the first time. I assume there will be a quite a few objects that are read once and never re-read. These objects don't have a T value attached to them. We could give them the average T over all the other objects. But then if the average T is > than 2.33 month then all first time objects would be evicted immediately, if otherwise all of them may remain there forever. 

% In general the problem here is that $T_{next}$ is only updated on reads, and what if a read never happens?
% So the problem is not solely with new objects - an object that is frequently read but then stops being read entirely is never evicted (because the $T_next$ of the object is never updated). }

}

\section{Additional Evaluation Results}\label{app:graphs}
This is a section that includes additional experiment results as mentioned in Section~\ref{s:eval}, including the results from cost savings on the 7-region setup with free placement mode (Figure~\ref{fig:7-region-fp}), and results from cost savings on 9-region setup with fixed base mode (Figure~\ref{fig:9-region-fb}). 
% \begin{figure*}[tbp]
%     \centering
%     \includegraphics[width=\textwidth]{figures/latency_9_region_no_base.pdf}
    
%     % \vspace{-2em}
%     \caption{\textbf{\sys Average Read Latency (ms) on 9-Region, Free Placement (FP)}: \sys.}
%     \label{fig:32trace-9region}
% \end{figure*}
